# Supplementary material for: C3Editor: Achieving Controllable Consistency in 2D Model for 3D Editing
Source: arXiv:2510.04539 source file (2025-10-31)
Supplement: Supplementary file 1 [file suppl_qualitative.pdf]

*"Give him a mustache"*

GT Image

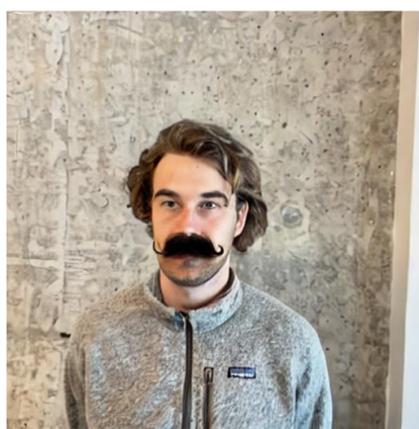

2D

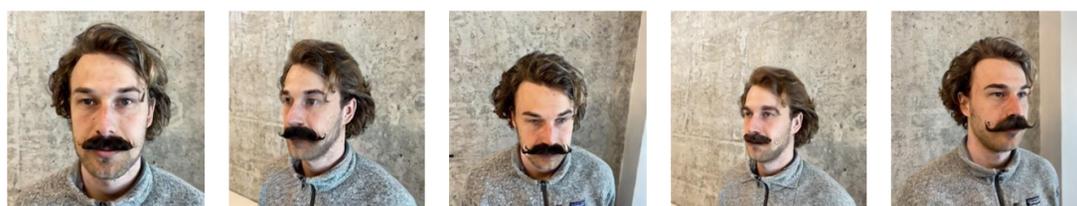

3D

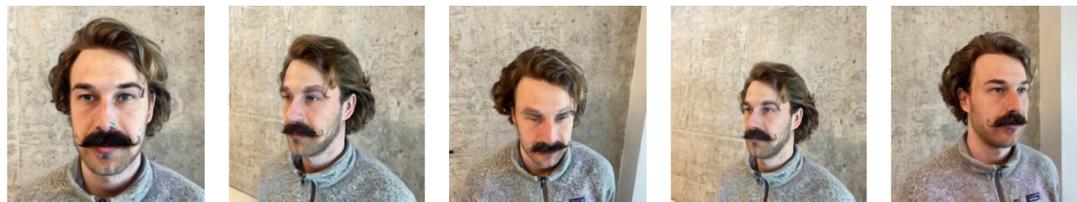

*"Give him a mustache"*

GT Image

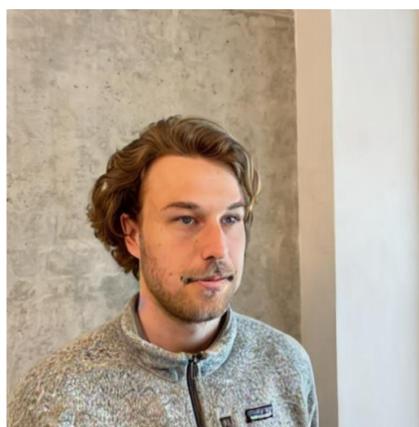

2D

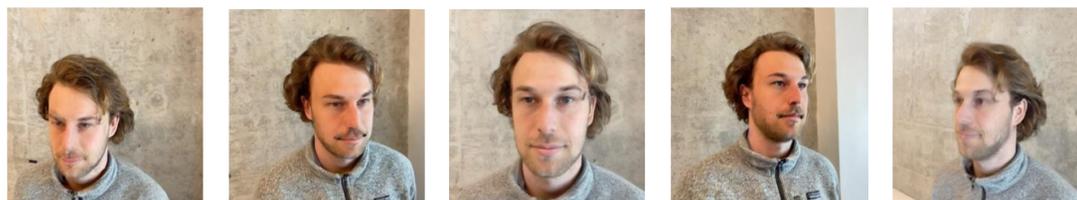

3D

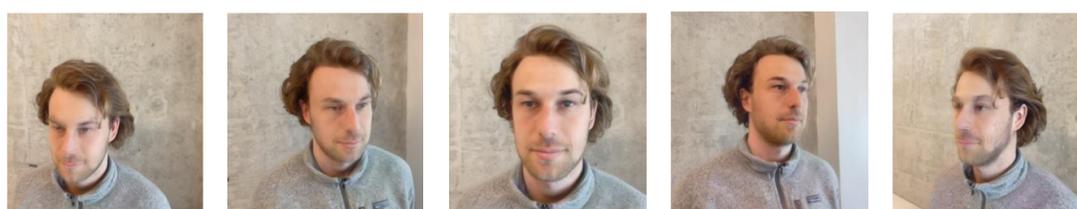

*"Turn him into a clown"*

GT Image

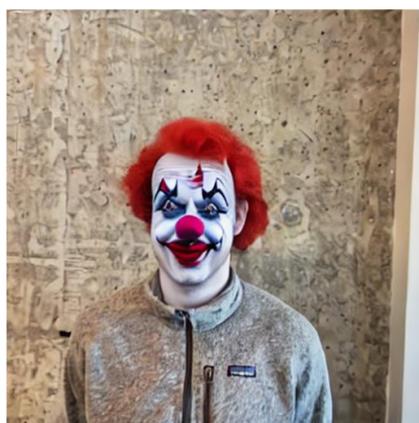

2D

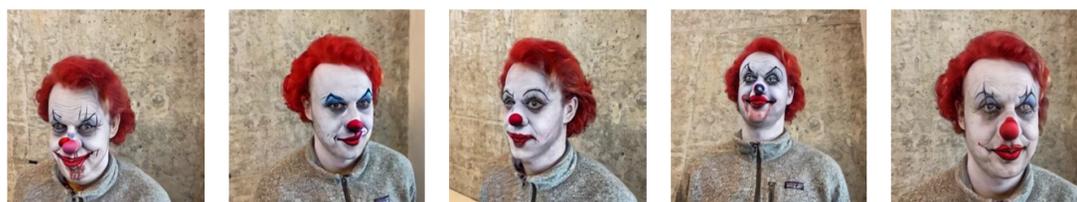

3D

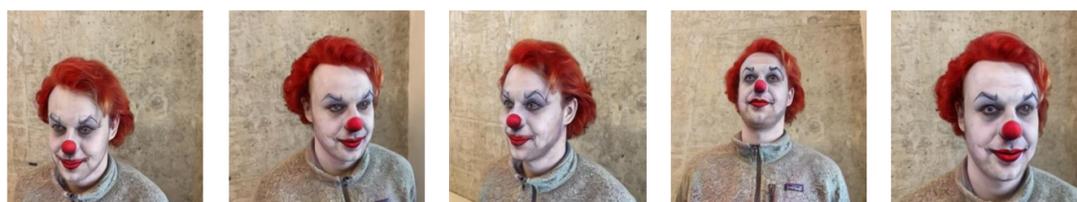

*"As a bronze bust"*

GT Image

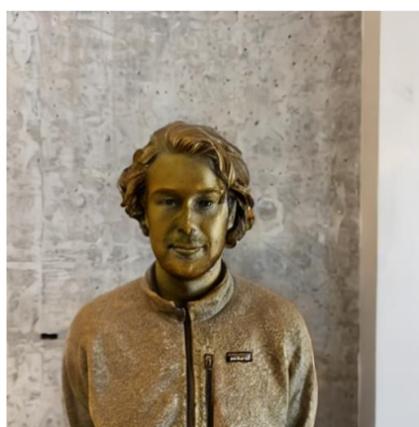

2D

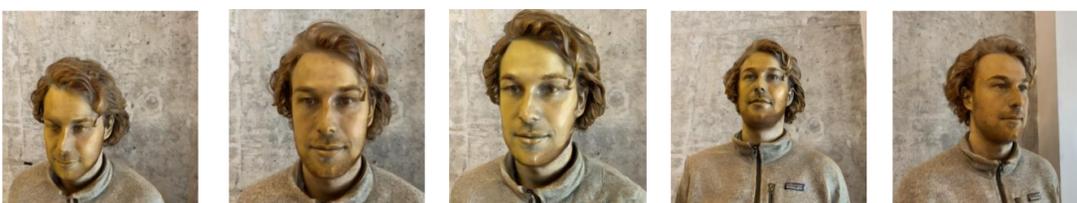

3D

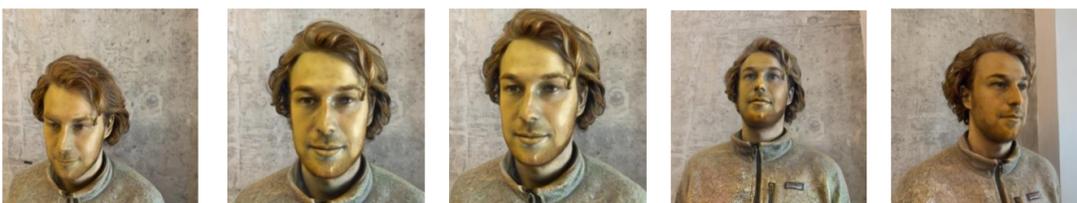

*"Make him bald"*

GT Image

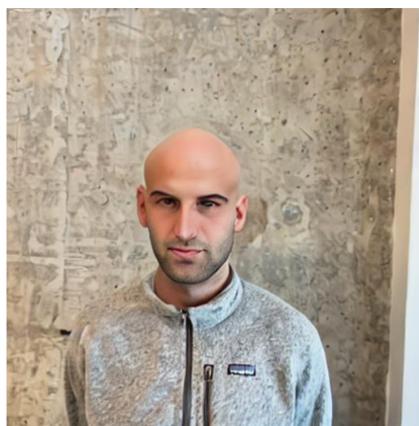

2D

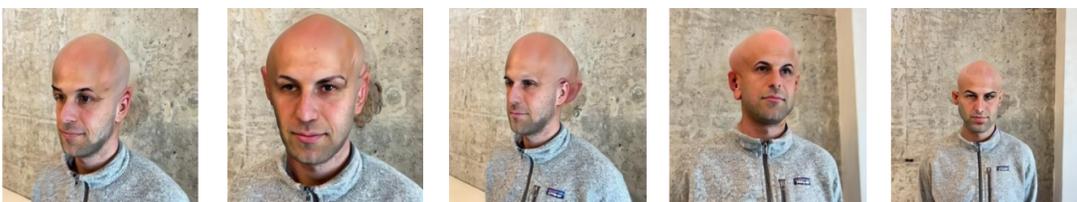

3D

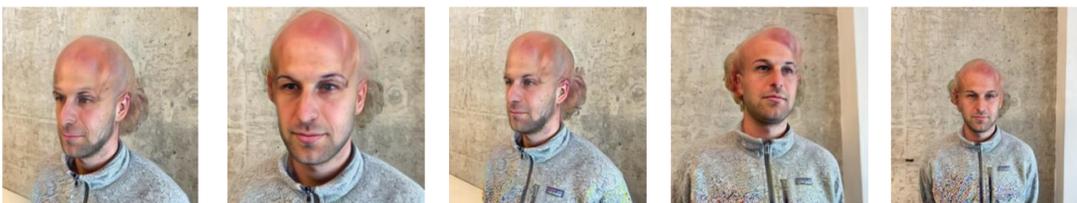

*"Turn him into Albert Einstein"*

GT Image

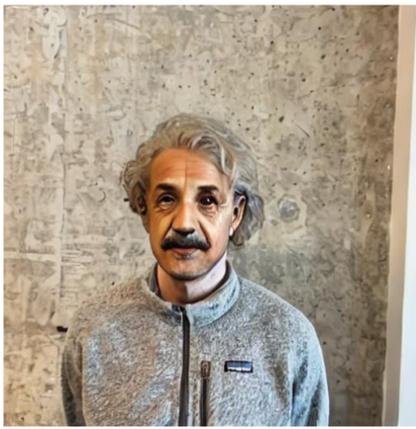

2D

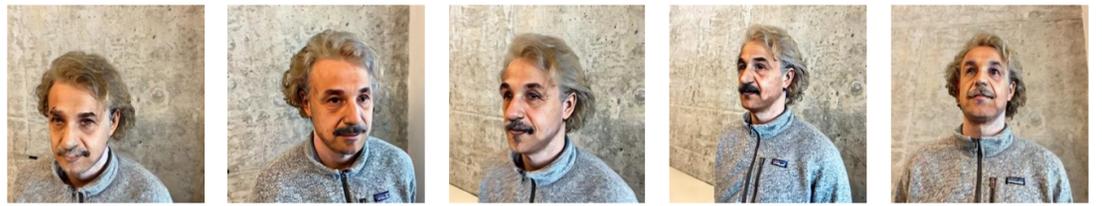

3D

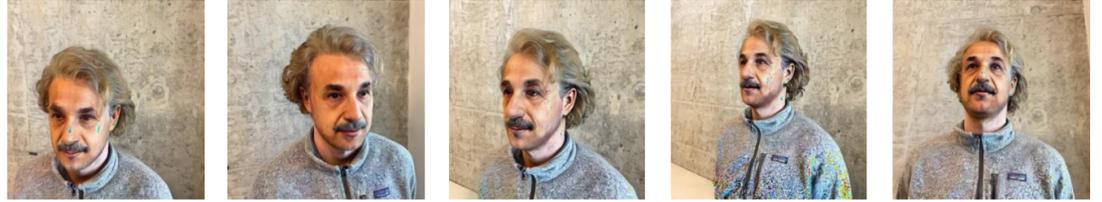

*"Customize the bench with a galaxy theme"*

GT Image

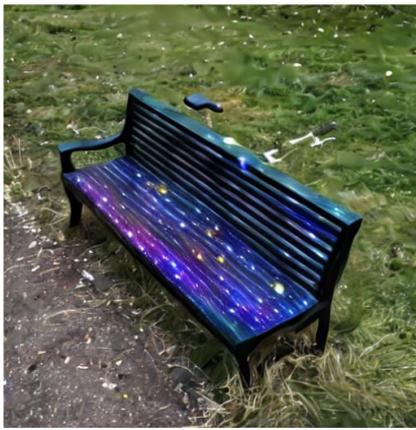

2D

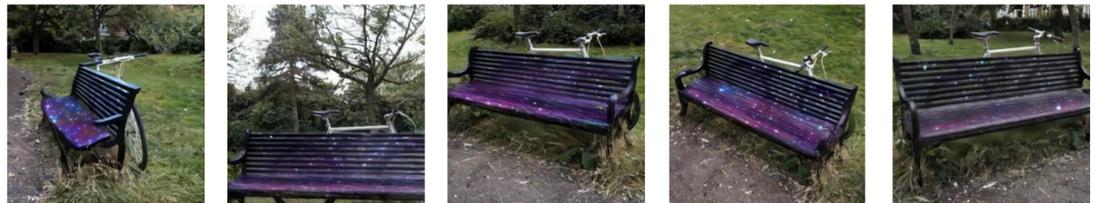

3D

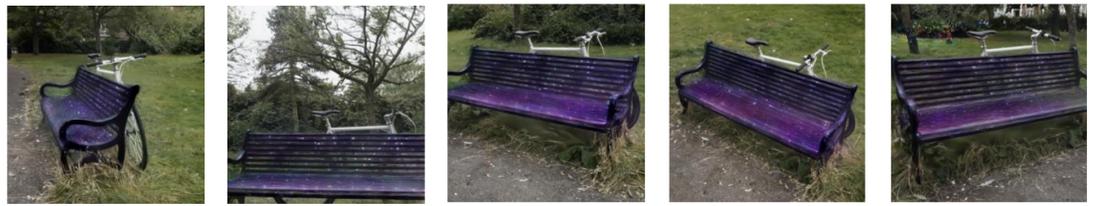

*"Add glowing lights around the bonsai branches"*

GT Image

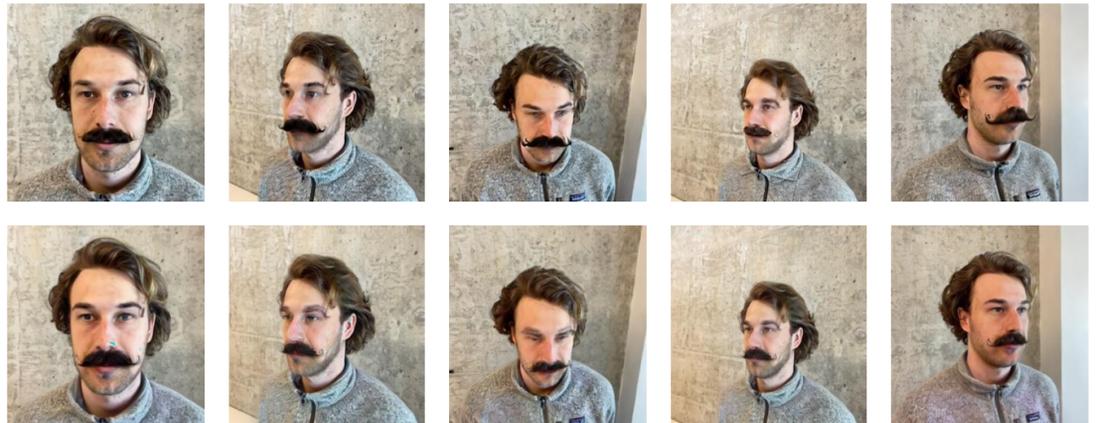

2D

3D

*"As a bronze bust"*

GT Image

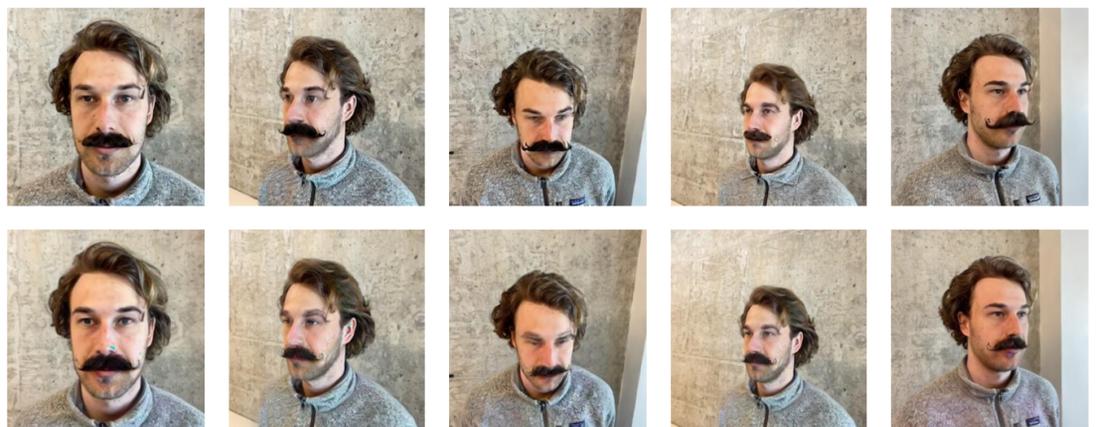

2D

3D

*"Make him bald"*

GT Image

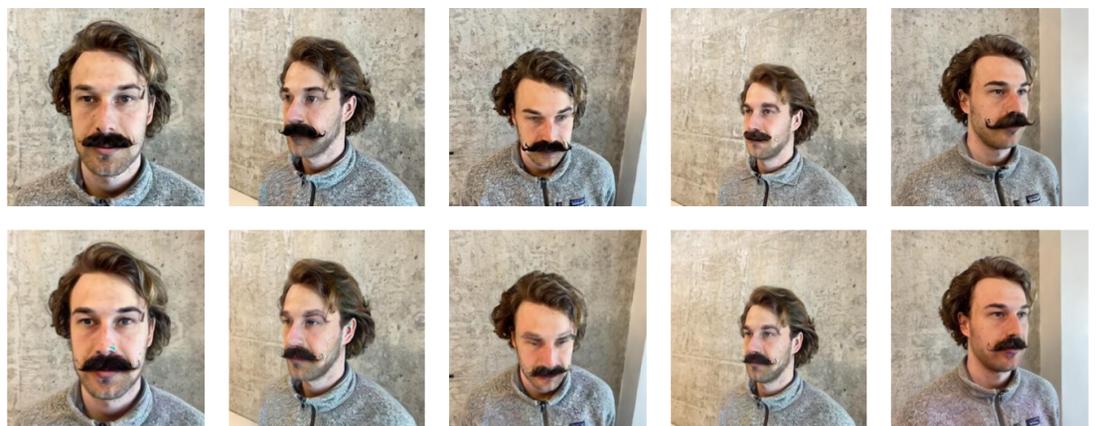

2D

3D
